# Supplementary material for: QCP: A Practical Separation Logic-based C Program Verification Tool
Source: arXiv:2505.12878 source file (2026-04-24)
Supplement: Supplementary file 1 [file AppendixB.tex]

\section{Example: LOS\_ListHeadInsert annotations}\label{appendixB}

Figure~\ref{fig:LosListHeadInsertFull} illustrates the use of \lstinline{which implies} to verify the function correctness of \lstinline{LOS_ListHeadInsert}. Similar to \lstinline{LOS_ListTailInsert}, here, we use the definitions \lstinline{dllseg_shift_rev}, whose definition is shown in Figure~\ref{fig:dllseg_shift_rev}. The formal definition is also provided below.

\begin{lstlisting}
dllseg_shift_rev(x,y,l) := x == y && l == nil && emp || 
                         exists z a l', l == cons(a, l') && 
                         x == snd a && x -> pstData == fst a &&
                         x -> pstNext == z && z -> pstPrev == x &&
                         dllseg_shift_rev(z, y, l')
\end{lstlisting}

\begin{figure}[!htp]
  \centering
  \inputminted[frame=lines,linenos]{c}{Figures/LOS_ListHeadInsertFull.list}
  \captionsetup{justification=raggedright, singlelinecheck=false}
  \caption{Annotations for \lstinline{LOS_ListHeadInsert}.}
  \label{fig:LosListHeadInsertFull}
\end{figure}

\begin{figure}[!htp]
  \centering
  \includegraphics[width=1\textwidth]{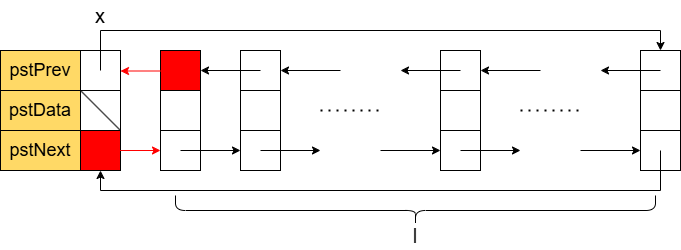}
  \captionsetup{justification=raggedright, singlelinecheck=false}
  \caption{The definition of predicate \lstinline{dllseg_shift_rev}. This predicate represents the memory structure depicted by the white area in the figure, which corresponds to the \lstinline{store_dll} structure excluding the red-highlighted portions.}
  \label{fig:dllseg_shift_rev}
\end{figure}
