# Supplementary material for: QCP: A Practical Separation Logic-based C Program Verification Tool
Source: arXiv:2505.12878 source file (2026-04-24)
Supplement: Supplementary file 2 [file AppendixE.tex]

\section{Example: Declarative and Operational Annotations}\label{appendixB}

This case study employs a queue formalized via a doubly-linked list to demonstrate the features from Section~\ref{DOA}. The predicate \lstinline{store_queue(q, l)} formally specifies queue structure \lstinline{q} with underlying data sequence \lstinline{l}. The \lstinline{queue} struct contains two pointer fields: \lstinline{head} and \lstinline{tail}, respectively referencing the list's endpoints, as formally defined below:
\begin{lstlisting}
struct dlist {
  int data;
  struct list *next;
  struct list *prev;
};

struct queue {
  struct list * head;
  struct list * tail;
};

/* store_queue(q, l) := dllseg(q->head,0,0,q->tail,l) */

/* dllseg(x,px,y,py,l) := x == y && px == px && l == nil && emp || 
    exists l0, l == cons(x->data, l0) && x -> prev == px && 
          dllseg(x->next,x,y,py,l0) */
\end{lstlisting}

The predicate definition of a doubly-linked list inherently requires only a single-direction unfolding, as the correctness of bidirectional access can be derived from this unidirectional specification. Through the verification of \lstinline{enqueue} and \lstinline{dequeue} operations, we demonstrate how our annotations unify declarative and operational reasoning.

In the verification of the \lstinline{enqueue} operation, we introduce two critical annotations: the \lstinline{which implies} annotation, which logically transforms the \lstinline{store_queue} predicate into a \lstinline{dllseg} to bridge the high-level queue abstraction with its low-level doubly-linked list representation, and the \lstinline{do dllseg_tail_unfold} annotation, which performs a tail-directed unfolding of the \lstinline{dllseg} predicate to enable precise structural reasoning from the tail node perspective.

\begin{lstlisting}
void enqueue(struct queue * q, int x)
  /*@ With l
      Require store_queue(q, l)
      Ensure store_queue(q, app(l, cons(x, nil)))
   */
{
  /*@ store_queue(q, l)
      which implies
      dllseg(q -> head, 0, 0, q -> tail, l) */
  struct list * p = malloc_list_cell();
  p -> data = x;
  if (q -> head == (void *)0) {
    q -> head = p;
    q -> tail = p;
    p -> next = (void *)0;
    p -> prev = (void *)0;
  }
  else {
    /*@ do dllseg_tail_unfold */
    q -> tail -> next = p;
    p -> prev = q -> tail;
    q -> tail = p;
    p -> next = (void *)0;
  }
}
\end{lstlisting}

\begin{lstlisting}
priority : dllseg_tail_unfold(1)
left : dllseg(?x,?px,?y,?py,?l) at 1
check : infer(x != y);
action : left_exist_add(l0);
         left_add(l == app(l0, cons(py->data, nil)));
         left_add(py->next == y);
         left_add(dllseg(x,px,py,py->prev,l0));
\end{lstlisting}

The \lstinline{do dllseg_tail_unfold} operation is a \emph{strategy-based operation}, requiring users to provide explicit Stellis strategies to guide its execution. Similar functionality can also be achieved using the \lstinline{which implies} annotation.
\begin{lstlisting}
/*@ q -> head != 0 && dllseg(q -> head, 0, 0, q -> tail, l)
    which implies
    exists l0, q -> tail != 0 && q -> tail -> next == 0 &&
      l == app(l0, cons(q -> tail -> data, nil)) &&
      dllseg(q -> head, q -> tail, 0, q -> tail -> prev, l0) */
\end{lstlisting}

The \emph{strategy-based operation} provides a general-purpose mechanism for fine-grained control in most scenarios, while \lstinline{which implies} is better suited for specialized cases, offering more flexible assertion transformation. This distinction is particularly evident in the \lstinline{dequeue} example: the first \lstinline{which implies} not only transforms \lstinline{store_queue} into \lstinline{dllseg} but also performs a head-directed unfolding of \lstinline{dllseg} based on the data list being \lstinline{cons(x, l)}.

\begin{lstlisting}
int dequeue(struct queue * q)
  /*@ With x l
      Require store_queue(q, cons(x, l))
      Ensure __return == x && store_queue(q, l)
   */
{
  /*@ store_queue(q, cons(x, l))
      which implies
      q -> head -> prev == 0 &&
      q -> head -> data == x &&
      dllseg(q -> head -> next, q -> head, 0 , q -> tail, l)
   */
  struct list * p = q -> head;
  int x0 = p -> data;
  q -> head = p -> next;
  free_list_cell(p);
  if (q -> head == (void *)0) {
    q -> tail = (void *)0;
  }
  else {
    /*@ do dllseg_head_unfold */
    q -> head -> prev = (void *)0;
  }
  return x0;
}
\end{lstlisting}

\begin{lstlisting}
priority : dllseg_head_unfold(1)
left : dllseg(?x,?px,?y,?py,?l) at 1
check : infer(x != y);
action : left_exists_add(l0);
         left_add(l == cons(x->data, l0));
         left_add(x->prev == px);
         left_add(dllseg(x->next,x,y,py,l0));
\end{lstlisting}
