# Supplementary material for: QCP: A Practical Separation Logic-based C Program Verification Tool
Source: arXiv:2505.12878 source file (2026-04-24)
Supplement: Supplementary file 3 [file AppendixH.tex]

\section{\wxw{Compare to Hip/Sleek}} \label{appendix:Hip}

Hip/Sleek is a verification tool for pointer-manipulating programs that uses bi-abduction and frame inference to solve separation logic entailments. 
%While it supports user-defined separation logic predicates, it lacks support for user-defined pure proposition predicates. The tool permits lemma definitions for separation logic predicates but not for pure propositions, making it incapable of achieving complete functional correctness proofs.
%In contrast, QCP allows users to define both functional predicates and separation logic predicates. For predicate operations, users can define strategies (similar to lemmas) for fold/unfold/other transformations, or perform declarative transformations through partial assertions or ``which implies`` clauses. QCP features an abduction-based separation logic solver for entailment elimination, while pure propositions are handled by an SMT solver. Any unprovable verification conditions are exported to Coq for manual proof, enabling QCP to support functional correctness proofs for arbitrary C programs.
We now examine specific Hip/Sleek features in detail:

\subsection{assertion with disjunctions} \label{hip:assertion}

While Hip/Sleek supports disjunctive assertions syntactically, it requires complete assertions in annotations (either as full assertions or multiple require/ensure clauses). QCP's multi-branch feature provides finer control - users can target specific branches for unfold/fold operations using \lstinline{$ branch_name} syntax without repeating operations across all branches. This granular control is absent in Hip/Sleek. See the section~\ref{hip:multi-specs} and \ref{hip:auto} examples for concrete demonstrations.

\subsection{multi-specs} \label{hip:multi-specs}
Hip/Sleek supports multiple specifications and their derivation relationships. However, during actual function calls, its solvers must identify applicable specifications automatically. QCP's \lstinline{where} clause explicitly specifies which specification to use during function calls, preventing redundant branching when multiple specifications' separation preconditions are satisfied but propositional parts cannot be verified by the SMT solver.

The concrete example can be found in the artifact \lstinline{QCP_benchmark/LiteOS/List_Add.c}. Our paper demonstrates the verification of \lstinline{LOS_ListTailInsert} and \lstinline{LOS_ListHeadInsert} using two \lstinline{which implies} clauses (Figure~\ref{fig:LosListTailInsertFull} and Figure~\ref{fig:LosListHeadInsertFull}) and one function specification (Figure~\ref{fig:LosListAdd}). 

We have modified this example as shown in Figure~\ref{fig:polyLOSList}, which presents the polymorphic version of \lstinline{LOS_ListAdd}'s specification. Unlike the specification in Figure~\ref{fig:LosListAdd}, we introduce a more concrete specification \lstinline{low_level_spec} that only involves specific memory addresses. The original specification becomes a derived specification \lstinline{high_level_spec}. Furthermore, the single data field is generalized to a polymorphic data field \lstinline{storeA}, removing restrictions on \lstinline{node} content. This example illustrates how QCP's multi-specification capability, combined with \lstinline{where} clauses, enables effective verification.

\begin{figure}[t]
  \centering
  \inputminted[frame=lines,linenos]{c}{Figures/poly_LOS_List.list}
  \vspace{-1.0em}
  \captionsetup{justification=raggedright, singlelinecheck=false}
  \caption{The multi-spec of \lstinline{LOS_ListAdd} for a polymorphic version.}
  \vspace{-1.0em}
  \label{fig:polyLOSList}
\end{figure}

Figure~\ref{fig:polyLOSListInsert} shows the annotations used in verification. In this implementation, the verification of \lstinline{LOS_ListHeadInsert} benefits from directly using \lstinline{high_level_spec}, which avoids unnecessary predicate folding/unfolding operations. Notably, this high-level specification demonstrates excellent reusability across similar invocation contexts. In contrast, \lstinline{LOS_ListTailInsert} utilizes the \lstinline{low_level_spec}, requiring predicate transformation through \lstinline{which implies} clauses.

\begin{figure}[t]
  \centering
  \inputminted[frame=lines,linenos]{c}{Figures/poly_LOS_Insert.list}
  \vspace{-1.0em}
  \captionsetup{justification=raggedright, singlelinecheck=false}
  \caption{The annotation of \lstinline{LOS_ListHeadInsert} and \lstinline{LOS_ListTailInsert} for a polymorphic version.}
  \vspace{-1.0em}
  \label{fig:polyLOSListInsert}
\end{figure}

Both functions utilize QCP's innovative \lstinline{where} clause mechanism for dynamic specification selection and logical parameter instantiation during function calls. While advanced separation logic solvers could handle the type parameter and polymorphic function instantiation in this example automatically, QCP's \lstinline{where} clause provides superior usability by offering developers explicit control over parameter specification, resulting in clearer proof structures and more maintainable verification processes.

\subsection{partial spec} \label{hip:partial-spec}

Hip/Sleek's partial specification feature (using annotations like \lstinline{@L}, \lstinline{@I}) allows users to specify invariant portions in require/ensure clauses. While similar to QCP's partial assertions, QCP offers greater flexibility by permitting partial assertions at any program point for needed transformations, with the frame automatically inferred by the separation logic solver.

\subsection{automatic fold/unfold/match inference rules} \label{hip:auto}

This feature resembles QCP's strategies, but QCP has \lstinline{which implies} clauses, enabling case-specific and declarative transformations without requiring general inference rules. To see how \lstinline{which implies} is useful in manual transformations, consider the following data structures and separation logic predicates.

\begin{figure}[t]
  \centering
  \inputminted[frame=lines,linenos]{c}{Figures/poly_queue.list}
  \vspace{-1.0em}
  \captionsetup{justification=raggedright, singlelinecheck=false}
  \caption{The definition of polymorphic singly-linked list}
  \label{fig:polysll}
\end{figure}

In this example, \lstinline{taskList} is a polymorphic single-linked list. The \lstinline{task_CB} predicate determines the data type stored in the list based on the \lstinline{taskStatus} field. We extend the basic singly-linked list predicate to \lstinline{sll(storeA,x,l)}, where \lstinline{storeA:} \{\lstinline{A}\} \lstinline{-> addr -> A -> Assertion} represents the memory information stored in list nodes. Since the actual information is stored in external fields, the starting node of sll needs to be computed through user-defined functions \lstinline{queue_entry}/\lstinline{mux_entry}/\lstinline{sem_entry} (corresponding to C functions \lstinline{Queue_entry}, \lstinline{Mux_entry}, and \lstinline{Sem_entry} respectively).

While Hip/Sleek can perform automatic entailment derivation for such cases, it requires separate predicate definitions for each type of \lstinline{sll}. QCP's \lstinline{which implies} allows manual case splitting/predicate decomposition for more flexible verification. For instance, in Figure~\ref{fig:polyqueue}, users want to prove the functional correctness of \lstinline{QueueUpdate}. Users first expand \lstinline{task_CB} along the \lstinline{QueueTask} branch using \lstinline{which implies}. During loop updates, strategies can unfold the \lstinline{sll} and \lstinline{queue_store} for complete updates. 

\begin{figure}[t]
  \centering
  \inputminted[frame=lines,linenos]{c}{Figures/poly_Queue.list}
  \vspace{-1.0em}
  \captionsetup{justification=raggedright, singlelinecheck=false}
  \caption{The annotation for verification of function \lstinline{QueueUpdate}}
  \vspace{-1.0em}
  \label{fig:polyqueue}
\end{figure}

\subsection{loop invariant vs. tail recursive call} \label{hip:loop}

Hip/Sleek can indeed transform loops into behaviorally equivalent tail recursive calls (using try-throw-catch) - an elegant and practical approach in many simple cases. However, this transformation doesn't actually reduce verification burden. For example, in VST-A's red-black tree case (Figure~\ref{fig:rbt}), even with recursive transformation, users must provide separate require/ensure for exit cases requiring multi-branch full assertions. QCP automatically computes exit assertions from loop invariants(Figure~\ref{fig:rbt_new}).

In summary, while Hip/Sleek shares several features with QCP, QCP introduces significant innovations and enhanced support in these areas.
