# Supplementary material for: QCP: A Practical Separation Logic-based C Program Verification Tool
Source: arXiv:2505.12878 source file (2026-04-24)
Supplement: Supplementary file 4 [file AppendixA.tex]

\section{Discussion: attempt of writing partial assertion in VeriFast}\label{appendixA}
This example in Fig~\ref{fig:VeriFast} is adapted from page 36 of the VeriFast tutorial (August 27, 2024)\cite{jacobs_2024_13380705}.
In this example, the \lstinline{assert} command in line 20 mechanically assigns logical variable names to the value of the predicate \lstinline{nodes} and the value of the field \lstinline{n->value}. These named values are then used in lines 24 and 25 to guide subsequent verification steps. While VeriFast appears to support functionality similar to partial assertions, its implementation is fundamentally limited to pattern matching: it merely matches structures within existing assertions and assigns names to corresponding values. 
\begin{figure}[!ht]
    \centering
    \lstinputlisting[linewidth={1\linewidth},frame=tb,basicstyle=\footnotesize\ttfamily,numbers=left,xleftmargin=2em]{Figures/VeriFast.list}
    \captionsetup{justification=raggedright, singlelinecheck=false}
    \caption{An examples of VeriFast}
    \label{fig:VeriFast}
\end{figure}
