# Supplementary material for: QCP: A Practical Separation Logic-based C Program Verification Tool
Source: arXiv:2505.12878 source file (2026-04-24)
Supplement: Supplementary file 5 [file AppendixG.tex]

Figure~\ref{fig:area} illustrates a rectangle area calculation example. The QCP IDE flags a proof goal at line 17, which concerns the multiplication validity of \lstinline{width * height} (i.e., \lstinline{INT_MIN <= width * height <= INT_MAX}). Based on the if-conditions at lines 11 and 14, we establish that both \lstinline{width} and \lstinline{height} range between 0 and 100, making this goal trivially valid. However, this constitutes a nonlinear verification problem that exceeds the capabilities of our built-in SMT solver, requiring nonlinear arithmetic support. By employing interval domain-based abstract interpretation, we can effectively resolve this issue through a simpler approach.

\begin{figure}
    \centering
    \vspace{-1.0em}
    \includegraphics[width=1\textwidth]{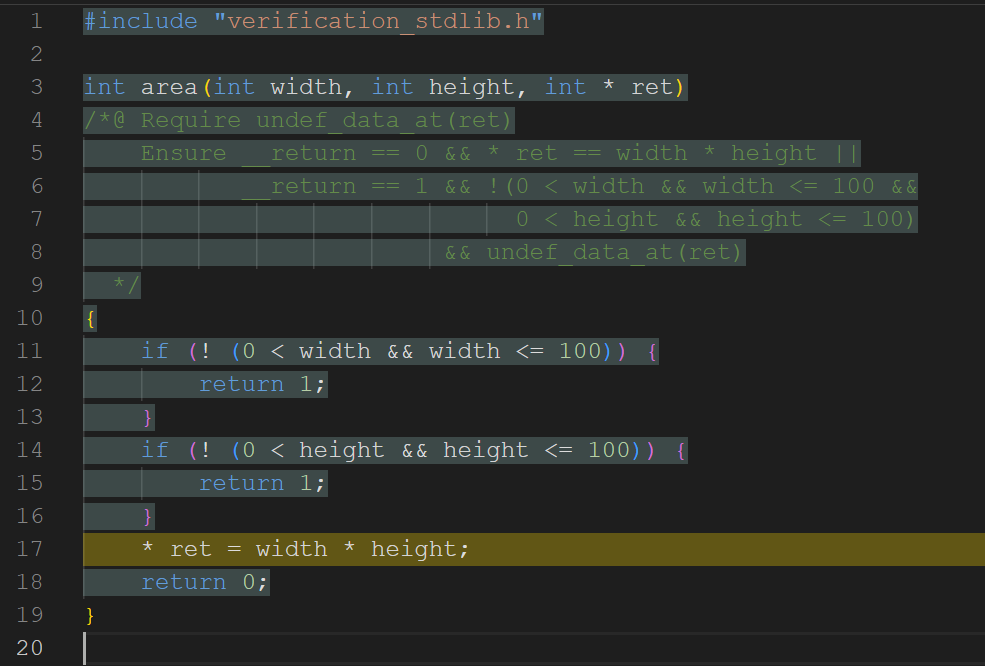}
    \captionsetup{justification=raggedright, singlelinecheck=false}
    \caption{An examples of function area}
    \label{fig:area}
\end{figure}
